# Supplementary material for: Synthesizing Abstract Transformers for Reduced-Product Domains
Source: arXiv:2408.04040 source file (2024-08-07)
Supplement: Supplementary file 1 [file appendix.tex]

\appendix
\section{Appendix}

% \subsection{Product domains: Direct and Reduced Products}
% \Cref{fig:diffRD} shows a variable \texttt{a} getting incremented thrice, and it also shows the abstract values in direct and reduced products of odd and even interval domain at each program point. \refline{code:diffinitD} and \refline{code:diffinitR} show the initial abstract value ($\mathtt{a^\sharp}$) of concrete value \texttt{a}. Initially $\mathtt{a^\sharp}$ represents the set $\{2,3,4\}$ ($\gamma(\mathtt{a^\sharp})$). \Cref{eq:incDirect} and \Cref{eq:incRed} show the direct and reduced transformers for increment operation, respectively. Application of direct and reduced transformers at each program point leads to the output shown in \refline{code:diffendD} and \refline{code:diffendR}. It is interesting to note that the $\gamma(a_3^{\sharp R}) \subset \gamma(a_3^{\sharp D})$ ($\{5,7\} \subset \{2,10\}$). Since abstract values are not shared across different domains, the direct product suffers from more imprecision than the reduced product.

\subsection{Abstract Domains}

\subsubsection{Interval Domain} 
Abstract values in this domain are of the form $[a, b]$, where $a$ is the low limit and $b$ is the upper limit. An interval $[a, b]$ represents the set of integer from $a$ to $b$. 

\subsubsection{Even Interval Domain}
This is an interval domain, with additional constraints of both limits being the even number. Interval $[a,b]$ is an even interval domain, only if $a\ mod\ 2\ =\ 0$ and $b\ mod\ 2\ =\ 0$.

\subsubsection{Odd Interval Domain}
Similar to the even interval domain, this also a variant of interval domain, where the end limits of interval $[a, b]$ are odd number, i.e., $a\ mod\ 2\ \neq\ 0$ and $b\ mod\ 2\ \neq\ 0$.

\subsection{Motivation Example}
%%%%%%%%%%%%%%%%%%%%%%%%%%%%%%%%%%%%%%%%%%%%%%%%%%%%%%%%%%%%%%%%%%
We use the increment operation (\texttt{++}) to explain each step of the \tool. \Cref{eq:incRed} shows the reduced transformer for the increment operator. \Cref{eq:intervalDSL} shows the domain-specific language (DSL) used to synthesize the reduced transformer for the odd-even domain. 

Our algorithm first initializes transformers for\evenintv and \oddintv with transformers shown in \Cref{eq:incDirect}. \tool iterates over each domain and tries to synthesize the sound and precise transformers for each domain. In this example, \tool starts with the odd interval domain (\oddintv).\tool will non-deterministically choose between soundness and precision checks, and in this case, \tool starts with the precision check and generates  $\langle\langle [-27, -25], [-28, -26]  \rangle, -24\rangle$ as a negative example and, the synthesized transformer for the \oddintv is shown below. 

\begin{align}
    \repo{inc}{o, e}_{\mathtt{odd}} = [\mathtt{min(-1, o.r), e.r+1}]
\end{align}

\tool invokes soundness and precision checks non-deterministically, generating negative and positive examples. A transformer refutes a negative example, and the examples satisfied by the transformers are the positive examples. 
Following is another transformer synthesized for \oddintv.

\begin{align}
    \repo{inc}{o,e}_{\mathtt{odd}} = [\mathtt{min(e.l - -1,  o.r), o.r}]
\end{align}

Since the above transformer is not sound, \tool emits $\langle\langle[27,29], [28, 30]\rangle, 30\rangle$ as the positive example during the soundness check.
The loop for synthesizing transformer for a single domain by generating positive and negative examples until \tool could synthesize a sound and precise transformer for \oddintv. \tool synthesizes the following transformer for the odd interval domain, which is a sound and precise transformer so far.

\begin{align}
    \repo{inc}{o,e}_{\mathtt{odd}} = [\mathtt{e.l + 1, e.r + 1}]
\end{align}

After generating a sound and precise transformer for \oddintv, \tool moves on to synthesizing transformers for the even interval domain (\evenintv). In the first iteration for \evenintv, \tool invokes precision check and generates a negative example, $\langle\langle[19, 23], [18, 22]\rangle, 19\rangle$. Similar to the \oddintv domain, \tool invokes a series of precision and soundness checks non-deterministically for \evenintv, and the following is the transformer synthesized for \evenintv, which is sound and precise so far. 

\begin{align}
    \repo{inc}{o,e}_{\mathtt{even}} = [\mathtt{o.l + 1, o.r + 1}]
\end{align}

Though we have generated sound and precise transformers for \oddintv in the previous iteration, the synthesis of transformers for \evenintv might affect the transformers for \oddintv. So, \tool will again iterate over both domains to check for the refinement of the current transformers. \tool checks for any refinement of the transformers for \oddintv, and both the soundness and precision check did not generate any example, marking transformers for \oddintv as sound and precise. Next,\tool checks for refinement of transformers for \evenintv, and similar to that of \oddintv, the synthesized transformer for\evenintv is sound and precise. As transformers for both domains are sound and precise, \tool emits \Cref{eq:incRed} as the final reduced transformer.

\subsection{End of section 3}
\subsection{Naive solutions for Product Domain transformers}

\begin{itemize}
  \item Scalable, precision may not be high
  \item Amurth runs on each domain separately
  \item challenges
\end{itemize}

\begin{align}
\dipt{add}{o_1, e_1}{o_2, e_2} &= \langle[\colorbox{red!20}{$e_1.l + e_2.l$},\ \colorbox{blue!20}{$e_1.r + e_2.r$}], \nonumber \\ &\hspace{7mm}[\colorbox{red!20}{$o_1.l + o_2.l - 1$},\ \colorbox{blue!20}{$o_1.r + o_2.r + 1$}]\rangle \label{eq:addDirect}
\end{align}

\Cref{eq:evenAddTrans} shows the transformer for the addition operation in \evenintv domain, whereas, \Cref{eq:oddAddTrans} shows the transformer for the same operation in \oddintv domain.

\subsubsection{Reduced Products}

\begin{itemize}
  \item High gain in precision, may not be scalable
  \item \amurth runs on product domain 
\end{itemize}

\subsubsection{Our Solution}
Cost similar to direct, precision similar to reduced

\subsection{Motivating example}
\label{sec:motivatingExample}

\subsection{Motivating example using addition}
\label{sec:motivatingExample}
In this section, we will be walking through an example to illustrate our reduced abstract transformers synthesis framework. In this example, we will be considering addition ($+$) operation to synthesize reduced transformers for even interval (\evenintv) and odd interval (\oddintv) abstract domain. \Cref{eq:evenAddOpt} and \Cref{eq:oddAddOpt} show one of the reduced transformers for the addition operation. 

\begin{align}
	\mathtt{add_{OR}^\sharp(\langle o_1, e_1\rangle, \langle o_2, e_2\rangle)} = [&\colorbox{red!20}{$\mathtt{max(o_1.l + e_2.l,\ o_2.l + e_1.l)}$},\nonumber \\& \ \colorbox{blue!20}{$\mathtt{min(o_1.r + e_2.r, o_2.r + e_1.r)}$}]\label{eq:evenAddOpt}\\
	\mathtt{add_{ER}^\sharp(o_1, e_1, o_2, e_2)} = [&\colorbox{red!20}{$\mathtt{max(o_1.l + o_2.l,\ e_1.l + e_2.l)}$},\nonumber \\ & \colorbox{blue!20}{$\mathtt{min(o_1.r + o_2.r, e_1.r + e_2.r)}$}]\label{eq:oddAddOpt}
\end{align}

Our algorithm starts with assigning $\bot$ to the both transformers of \evenintv and \oddintv. \tool iterates over each domain and tries to synthesize the sound and precise transformers for each domain. In this example, \tool starts with the odd interval domain (\oddintv). At first soundness check fails as the current transformer is $\bot$ and emits $\langle\langle [-31, 1, -30, 0], [-31, 1, -30, 0]\rangle, -60 \rangle$ as the positive example. Positive examples are the set of examples which should be satisfied by the transformers. These positive examples are being used in each synthesis call. In the next iteration, \tool will call for a precision check along with the generated positive example. \tool generated $\langle\langle[-15, -13, -14, -14],\ [-31, -29, -30, -28]\rangle, 1  \rangle$ as the negative example and following is the synthesized transformer. 

\begin{align*}
	\mathtt{add_{OR}^\sharp(o_1, e_1, o_2, e_2) =}& [\colorbox{red!20}{$\mathtt{min(0, e_2.l + e_2.l)-1}$},\colorbox{blue!20}{$\mathtt{ o_2.r+1}$}]
\end{align*}

Similarly, the \tool keeps on generating both negative and positive examples using precision and soundness check, respectively. The loop for synthesizing transformer for a single domain by generating positive and negative example until \tool could synthesize a sound and precise transformer for \oddintv. \tool synthesizes following transformer for odd interval domain which is sound and precise transformer so far. 

\begin{align}
	\mathtt{add_{OR}^\sharp(o_1, e_1, o_2, e_2) =}& [\colorbox{red!20}{$\mathtt{max(o_2.l + e_1.l,\ o_1.l + e_2.l)}$}\nonumber \\
	&\ \colorbox{blue!20}{$\mathtt{max(o_1.r + o_2.r,\ e_1.r + e_2.r) - 1}$}]\label{eq:oddAddSynthesized}
\end{align}

After generating a sound and precise transformer for \oddintv, \tool moves on to the synthesis of transformers for even interval domain (\evenintv).
In the first iteration for \evenintv, \tool invokes precision check and generated following negative example, $\langle\langle[11, 21, 10, 20], [-25, -23, -26, -24]\rangle, -15\rangle$. Similar to the \oddintv domain, \tool invokes a series of precision and soundness checks non-deterministically for \evenintv too. Following is the transformer synthesized for \evenintv which is sound and precise so far. 

\begin{align}
\mathtt{add_{ER}^\sharp(o_1, e_1, o_2, e_2) =}& [\colorbox{red!20}{$\mathtt{max(o_1.l + o_1.l,\ e_1.l + e_2.l)}$}\nonumber \\
&\ \colorbox{blue!20}{$\mathtt{max(o_1.r + e_2.r,\ o_2.r + e_1.r) - 1}$}] \label{eq:evenAddSynthesized}
\end{align}

Though we have generated sound and precise transformers for \oddintv in the previous iteration, but, synthesis of transformers for \evenintv might affect the transformers for \oddintv. So, we will again iterate over both domains to check for the refinement of the current transformers. Now, \tool check for any refinement of the transformers for \oddintv, and both the soundness and precision check did not generate any example, marking transformers for \oddintv as sound and precise. In the next iteration \tool moves to synthesize transformers for \evenintv, and similar to that of \oddintv, \tool could not find any refinement of transformers for \evenintv. As transformers for both domains is sound and precise, \tool emits \Cref{eq:evenAddSynthesized} and \Cref{eq:oddAddSynthesized} as the final transformers. These transformers are equivalent to the \Cref{eq:evenAddOpt} and \Cref{eq:oddAddOpt}. 

\todo{PK: will add proof}

\subsection{Naive combination: challenges}

\subsection{Our algorithm}
